# Supplementary material for: Accurate Lindblad-Form Master Equation for Weakly Damped Quantum Systems Across All Regimes
Source: arXiv:1906.08279 source file (2020-02-28)
Supplement: Supplementary file 1 [file supplement.pdf]

# Supplement: Accurate Lindblad-Form Master Equation for Weakly-Damped Quantum Systems Across All Regimes

Gavin McCauley,[1] Benjamin Cruikshank,[1,2] Denys I. Bondar,[3] and Kurt Jacobs[1,2,4]

[1]*U.S. Army Research Laboratory, Computational and Information Sciences Directorate, Adelphi, Maryland 20783, USA*
[2]*Department of Physics, University of Massachusetts at Boston, Boston, MA 02125, USA*
[3]*Department of Physics and Engineering Physics, Tulane University, New Orleans, LA 70118, USA*
[4]*Hearne Institute for Theoretical Physics, Louisiana State University, Baton Rouge, LA 70803, USA*

Here we show comparisons between the master equation derived in the main text, exact simulations, and the Bloch-Redfield equation. We also give the degenerate and non-degenerate Lindblad-form master equations, and explicit expressions for all the Hamiltonians and transition operators of the systems depicted in Fig.1 in the main text.

## I. COMPARISON WITH THE BLOCH-REDFIELD EQUATION

In the main text we compared the Linblad-form master equation we derived, Eq.(37), to exact simulations for various systems coupled to an Ohmic bath. Here we confirm, using the V system as an example, that the Linblad-form master equation is very close to the Bloch-Redfield equation, and both have essentially the same accuracy with regard to the exact evolution. For these comparisons we use the same parameters for the V system as used for Fig.2 in the main text, and we use the same measure for the difference between the predicted evolutions. First, in Fig.1, we plot the difference between our Linblad-form equation and the B-R equation for three values of the detuning, $\Delta\omega = \gamma$, $4\gamma$, and $100\gamma$. Second, in Fig.2, we plot the discrepancy between our master equation and the exact simulations (red) and between the B-R equation and the exact simulations (blue), for the same three values of the detuning. We see from Fig.2 that the accuracy of our master equation and the B-R equation are essentially the same. We see also from Fig.1 that the difference between the evolution of the B-R equation and our equation is less than that between either of them and the exact evolution for the Ohmic bath.

## II. THE LINDBLAD MASTER EQUATIONS FOR THE DEGENERATE AND NON-DEGENERATE REGIMES

Define $N$ "transition operators", $\sigma_j, j = 1, 2, \ldots, N$, in which $\sigma_k$ transforms the upper state of transition $k$ to its lower state. Also let us denote the frequency and decay rate of transition $j$ by $\omega_j$ and $\gamma_j$, respectively, and define

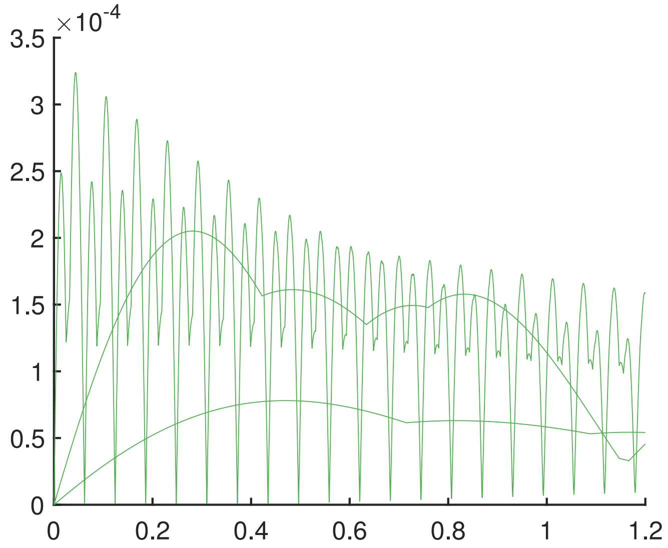


FIG. 1. (Color online) A measure of the difference between the evolution of the master equation we derive in the main text and that of the B-R equation, for the V system using the parameters of Fig.2 in the main text, for three values of the detuning: $\Delta\omega = \gamma$, $4\gamma$, and $100\gamma$.

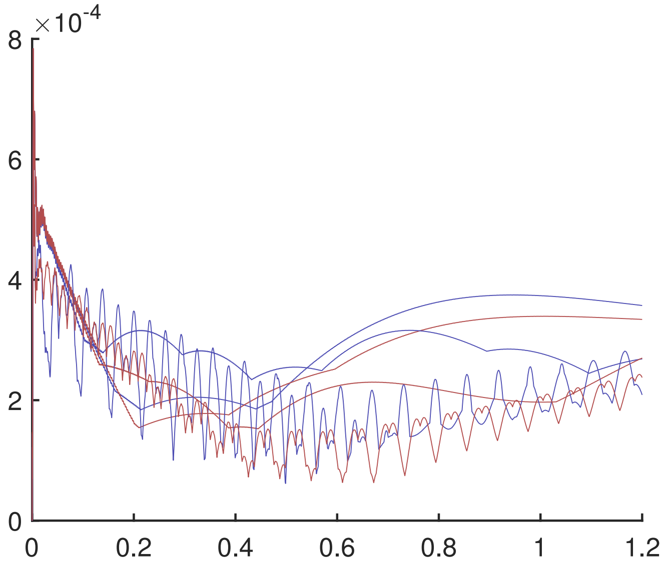


FIG. 2. (Color online) (Color online) A measure of the accuracy of the master equation we derive in the main text (red) and that of the B-R equation (blue), for the V system using the parameters of Fig.2 in the main text, for three values of the detuning: $\Delta\omega = \gamma$, $4\gamma$, and $100\gamma$.

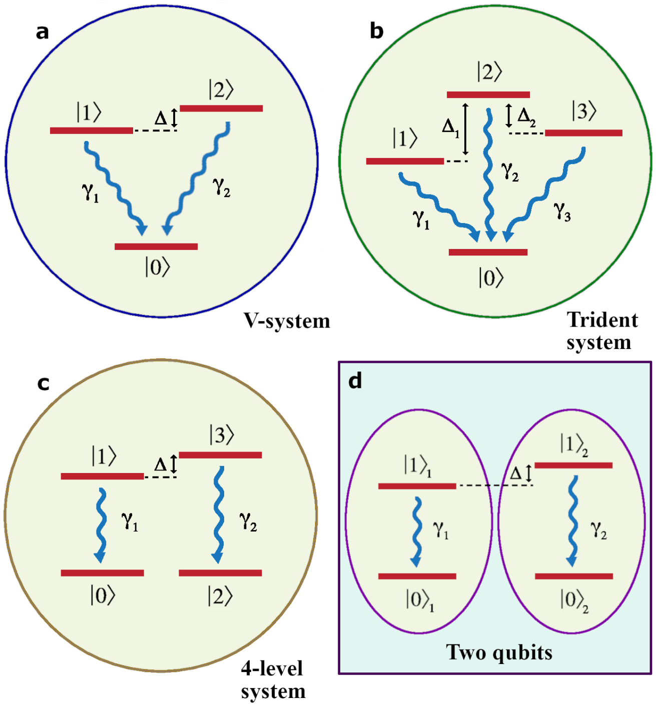


FIG. 3. (Color online) Here we reproduce the diagram of Fig.1 in the main text that shows the four systems for which we perform numerical simulations.

the "super operator" $\mathcal{D}$ by

$$\mathcal{D}[c]\rho \equiv \tfrac{1}{2}\left(c^\dagger c\rho + \rho c^\dagger c - 2c\rho c^\dagger\right). \quad (1)$$

*The non-degenerate master equation:* If the transitions are non-degenerate ($|\omega_j - \omega_k| \gg \max(\gamma_j,\gamma_k)$, $\forall j,k$), the master equation that describes their evolution at zero temperature is

$$\dot\rho = -\frac{i}{\hbar}\left[H_0 - \hbar\sum_j \Delta_L^{(j)}\sigma_j^\dagger\sigma_j,\rho\right] - \sum_j \gamma_j\mathcal{D}[\sigma_j]. \quad (2)$$

Here the Lamb-shift to the frequency of each transition can be written as $\Delta_L^{(j)} = f(\omega_j)\gamma_j$ (see Eq.(42) in the main text). This is a convenient way to write it for the degenerate master equation below. The non-degenerate master equation is characterized by having independent photon decays between different transitions. another way to put this is that different transitions are effectively coupled to different baths, so that the bath does not induce interactions between the transitions.

*The degenerate master equation:* When $\omega_j = \omega$, $\forall j$, the master equation is instead

$$\dot\rho = -\frac{i}{\hbar}\left[H_0 - \hbar f(\omega)\Sigma^\dagger\Sigma,\rho\right] - \mathcal{D}[\Sigma]\rho, \quad (3)$$

in which

$$\Sigma = \sum_j e^{i\phi_j}\sqrt{\gamma_j}\sigma_j, \quad (4)$$

and $\phi_j$ is determined by the phases of the interactions between the transitions and the bath (see Eq.(9)). Note that if $\sigma_j^\dagger\sigma_k$ does not vanish, the Lamb-shift Hamiltonian for the degenerate master equation, $H = \hbar f(\omega)\Sigma^\dagger\Sigma$, includes a coherent effective interaction between the upper levels of transitions $j$ and $k$. If the transitions belong to different atoms, then this interaction is the dipole contribution to the force between the atoms [1]. The degenerate master equation contains all the terms of non-degenerate master equation, plus additional terms that involve pairs of transitions.

## III. EXPRESSIONS FOR HAMILTONIANS AND TRANSITION OPERATORS

The master equations given in Eqs.(37) and (50) of the main text contain transition operators $\sigma_j$ and transition frequencies $\omega_j$. For reference we give here the explicit expressions for the transition operators and frequencies for all the systems that we define in Fig.1 of the main text (reproduced below as Fig.3). Let us denote the energy of state $|j\rangle$ by $E_j$, so that the Hamiltonian for every system in Fig.3 can be expressed as

$$H_{\rm sys} = \sum_j E_j|j\rangle\langle j|. \quad (5)$$

With these definitions the transition operators and frequencies for each of the systems in Fig.3 are as follows.

Three-level V-system:

$$\omega_j = (E_j - E_0)/\hbar, \quad (6)$$
$$\sigma_j = |0\rangle\langle j|, \quad j = 1,2. \quad (7)$$

Three-transition "trident" system:

$$\omega_j = (E_j - E_0)/\hbar, \quad (8)$$
$$\sigma_j = |0\rangle\langle j|, \quad j = 1,2,3. \quad (9)$$

Four-level system:

$$\omega_1 = (E_1 - E_0)/\hbar, \quad (10)$$
$$\sigma_1 = |0\rangle\langle 1|, \quad (11)$$
$$\omega_2 = (E_3 - E_2)/\hbar, \quad (12)$$
$$\sigma_2 = |2\rangle\langle 3|. \quad (13)$$

Pair of qubits:

$$H_0 = E_1\left(|1\rangle\langle 1|\otimes I\right) + E_2\left(I\otimes|1\rangle\langle 1|\right), \quad (14)$$
$$I \equiv |0\rangle\langle 0| + |1\rangle\langle 1|, \quad (15)$$
$$\omega_1 = E_1/\hbar, \quad (16)$$
$$\omega_1 = E_2/\hbar, \quad (17)$$
$$\sigma_1 = |0\rangle\langle 1|\otimes I, \quad (18)$$
$$\sigma_2 = I\otimes|0\rangle\langle 1|. \quad (19)$$

[1] Fam Le Kien, S. Dutta Gupta, K. P. Nayak, and K. Hakuta, "Nanofiber-mediated radiative transfer between two distant atoms," Phys. Rev. A **72**, 063815 (2005).
